# Supplementary material for: Element-Specific Depth Profile of Magnetism and Stoichiometry at the La0.67Sr0.33MnO3/BiFeO3 Interface
Source: arXiv:1407.0737 ancillary file (2014-07-02)
Supplement: Supplementary file 1 [file supplemental-material.pdf]

Supplemental Material

# Element-Specific Depth Profile of Magnetism and Stoichiometry at the $La_{0.67}Sr_{0.33}MnO_3/BiFeO_3$ Interface

J. Bertinshaw,[1,2] S. Brück,[1,2] D. Lott,[3] H. Fritzsche,[4] Y. Khaydukov,[5] O. Soltwedel,[5] T. Keller,[5] E. Goering,[6] P. Audehm,[6] D. L. Cortie,[2] W. D. Hutchison,[7] Q. M. Ramasse,[8] M. Arredondo,[9] R. Maran,[10] V. Nagarajan,[10] F. Klose,[2,11] and C. Ulrich[1,2]

[1]*School of Physics, The University of New South Wales, Sydney, NSW 2052, Australia*

[2]*Australian Nuclear Science and Technology Organisation, Lucas Heights, NSW 2234, Australia*

[3]*Institute for Materials Research, Helmholtz Zentrum Geesthacht, 21502 Geesthacht, Germany*

[4]*Canadian Neutron Beam Centre, Chalk River Laboratories, Ontario K0J 1J0, Canada*

[5]*Max-Planck-Institute for Solid State Research, outstation FRM II, D-70569 Stuttgart, Germany*

[6]*Max-Planck-Institute for Intelligent Systems, D-70569 Stuttgart, Germany*

[7]*School of Physical, Environmental and Mathematical Sciences, The University of New South Wales, Canberra, ACT 2600, Australia*

[8]*SuperSTEM Laboratory, STFC Daresbury Campus, Keckwick Lane, Daresbury WA4 4AD, UK*

[9]*School of Mathematics and Physics, Queen's University Belfast, Belfast BT7 1NN, UK*

[10]*School of Materials Science and Engineering, The University of New South Wales, Sydney, NSW 2052, Australia*

[11]*Department of Physics and Materials Science, City University of Hong Kong, Hong Kong, SAR China*

# I. SUPPORTING DOCUMENTS: SCANNING TRANSMISSION ELECTRON MICROSCOPY AND ELECTRON ENERGY LOSS SPECTROSCOPY

Analytical scanning transition electron microscopy (STEM) and electron energy loss spectroscopy (EELS) were performed on samples grown under identical conditions as presented in the main text in order to assess interface quality and chemical composition over a small cross-sectional area, providing supporting evidence of the results of the PNR and resonant XRR studies presented in the main text. The TEAM 0.5 microscope, an optimised double aberration-corrected FEI Titan3 instrument operated at 300 kV acceleration voltage, was used to acquire high angle annular dark field (HAADF) images, whose contrast offers high sensitivity to variations between atomic species. In optimal conditions, this microscope creates a 0.5 Å STEM probe (full-width at half-maximum) [1]. The convergence semi-angle of the electron probe used to record the images presented here was 32 mrad, with a probe current of 60 pA. The inner and outer radii of the HAADF detector were measured as 65 mrad and 350 mrad respectively in the imaging conditions. In the HAADF image presented in Fig. 1, the contrast scales to a good approximation with the square of the atomic number Z (so-called 'Z-contrast mode'), providing a visual means of identifying qualitatively the position of the interface between the lighter LSMO and heavier BFO. When taking different images across the sample, the interface appears to be perfectly coherent over a large distance, with subtle Z-contrast variations suggesting an interface roughness of ∼5 Å i.e. of about 1 and 2 octahedral sites over the entire sample. This is in accordance with our XRR studies presented in the main text.

The results of the EELS mapping is shown in Fig. 2. It reveals a gradient of sub-stoichiometry in the Mn- and O-ions within the first 2 nm at the $La_{0.67}Sr_{0.33}MnO_3/BiFeO_3$ interface, supporting the results and analysis performed in the main text. EELS linescans were performed at additional regions with reproducible results. The same sample was used for both the STEM and the EELS studies. EELS chemical mapping was carried out on a dedicated aberration-corrected Vacuum Generators (VG) HB501 STEM, operated at 100 kV. The probe-forming optics were adjusted to form a ∼1.1 Å beam, with 22 mrad convergence semi-angle and a current of 80 pA. The HAADF detector inner and outer radii were calibrated at 72 mrad and 210 mrad respectively, while EELS spectra were recorded with a Gatan Enfina spectrometer through a 18.5 mrad semi-angle collection aperture. Although

the instrument has a native energy resolution of 0.3 eV, to cover the spectral dispersion to measure energy loss from the onset of the O K edge (532 eV) to the La $M_{4,5}$ edge (830 eV), the effective energy resolution was ∼0.8 eV, limited by the detector point spread function. Because of the lower acceleration voltage, a thinner area of the sample was necessary for the EELS study, which was estimated from low loss EELS data [2] as approximately 10-20 nm. The EELS data was de-noised using principal component analysis [3].

It should be noted that in order to quantify the results of the atomic resolution EELS mapping, the STEM images and full quantitative simulations of both imaging and spectroscopy data need to be considered to account for EELS delocalisation effects [4]. Oxygen modifications are difficult to visualize and quantify using STEM and EELS due to the low Z-contrast of the light O-ions. However, the combined results of local probe mapping using STEM and EELS clearly support the conclusion given in the main text that the interfacial region of an altered stoichiometry and is mainly located within the LSMO layer and has a width of about 2 nm. By using advanced synchrotron and neutron reflectometry techniques, as presented in the main text, the relationship between the observed reduced magnetization in the intermediate layer is discussed in terms of oxygen vacancies in the interfacial region.

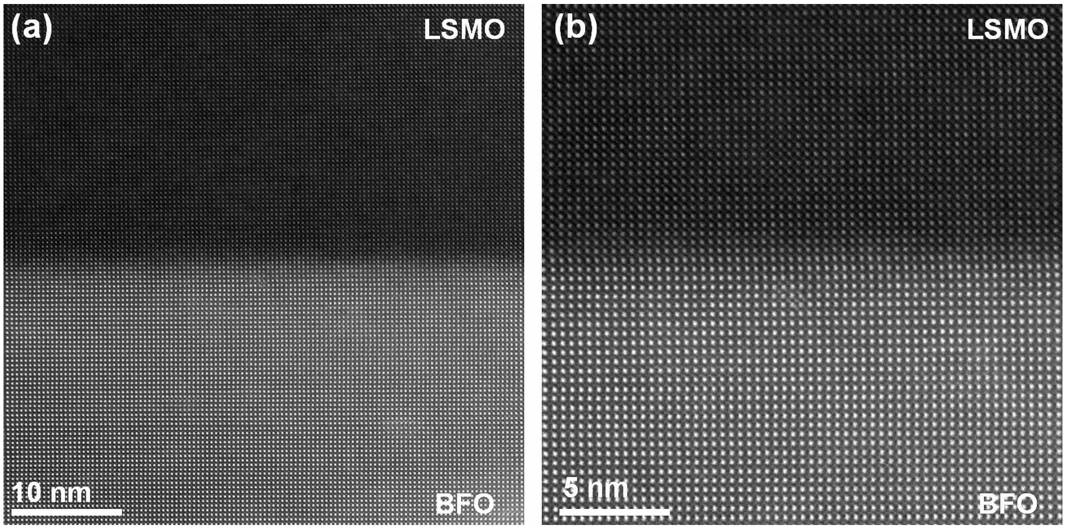


FIG. 1. HAADF (Z-contrast) images of the $La_{0.67}Sr_{0.33}MnO_3/BiFeO_3$ interface acquired on the TEAM0.5 electron microscope at 300 kV acceleration voltage. The interface appears perfectly coherent over large distances, indicating the high structural quality of the bi-layer interface.

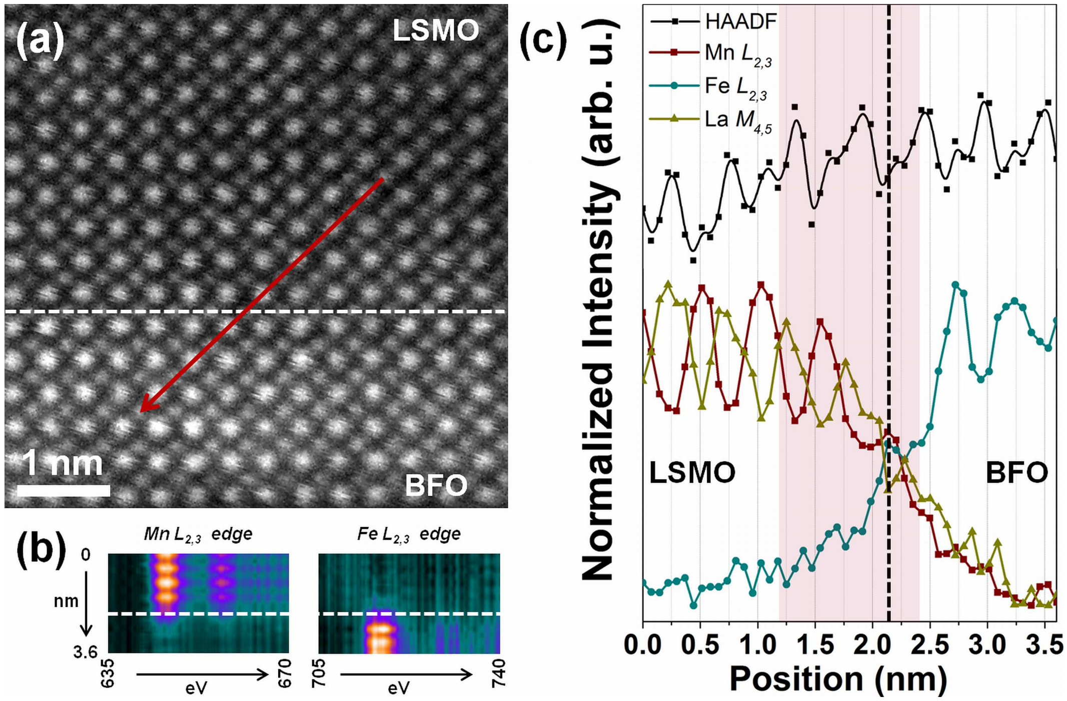


FIG. 2. a) HAADF image of the $La_{0.67}Sr_{0.33}MnO_3/BiFeO_3$ interface in a very thin region of the sample. The white dotted line is a guide to the eye for the interface position. b) A 1-dimensional EELS linescan was acquired across the interface along the direction shown by the red arrow in (a). The Mn and Fe $L_{2,3}$ edge regions of the EELS data show a clear oscillatory contrast, confirming atomic resolution. The dotted lines correspond to the interface position marked in (a). c) Chemical profiles obtained by integrating the EELS intensity over a 35 eV window above the respective energy onsets of the Mn $L_{2,3}$, Fe $L_{2,3}$ and La $M_{4,5}$ edges. The intensities are normalized for clarity. The HAADF intensity was recorded simultaneously to the EELS data. A vertical dotted line indicates the interface position. Importantly, a 2 nm region within the $La_{0.67}Sr_{0.33}MnO_3$ side of the interface appears to be sub-stoichiometric, whereas no such gradient is found on the $BiFeO_3$ side. This region is highlighted by a red shadow in (c).

## II. MAGNETOMETRY AND POLARIZED NEUTRON REFLECTION TEMPERATURE DEPENDENCY STUDIES

Magnetization measurements were performed on PPMS and MPMS setups (company Quantum Design) for the thin film bi-layer samples presented in the main text, in order to accurately characterize the overall magnetization of the films. Figure 3 presents hysteresis curves measured at different temperatures, whereas Fig. 4 presents the field cooled magnetization temperature dependence of the system, with an applied field of 20 mT. These results are in general accordance with previous literature magnetization properties of thin film LSMO deposited by Pulsed Laser Deposition on (001)-oriented $SrTiO_3$ substrates (see refs. [15, 17, 18] in the main text). The magnetic moment parameter of the LSMO layer determined through analysis of the PNR reflectivity curves performed on the instruments NREX and Platypus with an applied field of 0.1 mT was found to be in close agreement with the overall magnetic moment determined through magnetometry (Fig. 1 in the main text).

Figure 4 shows a comparison of the magnetization values obtained by magnetometry (black squares) and those fitted to data of the LSMO interface layer (blue circles) as determined from a temperature dependency PNR experiment performed on the instrument D3 at NRU, Chalk River, Canada. For the fitting process, the magnetic moment of the bulk of the LSMO layer (red diamonds) was derived from the magnetometry data, and the thickness of the interface layer was fixed to 26 Å. For the experiment, full saturation of the LSMO Mn-ion magnetic moment was achieved by field cooling and measuring under an applied field of 3 T. From the extrapolation of the magnetometry data, a magnetic transition $T_C \approx 345(5)$ K was obtained for the bulk of the film. This is in accordance to previous experiments (see refs. [15, 18, 19, 20] given in the main text). We have further extrapolated the moment of the interfacial layer and obtained a reduced $T_C$ of $\approx 316(10)$ K, a reduction of around 30 K. The analysis of our polarized neutron reflectometry data further indicated a reduction of the magnetic moment of about 40 % and remains constant with temperature. This reduction is discussed in the main text as mainly being caused by an altered stoichiometry in this interfacial region.

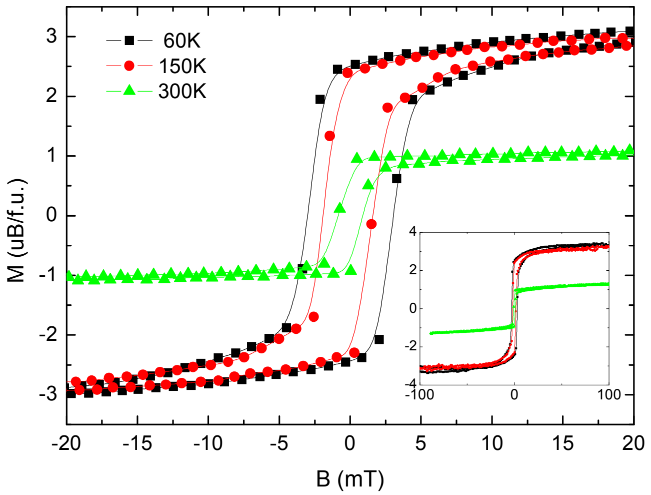


FIG. 3. Magnetic hysteresis loops measured at 60 K, 150 K and 300 K. The inset shows the extended loop taken at 150 K. The saturation moment is less than that of bulk LSMO, and the hysteresis shape is not completely square, indicating magnetic anisotropy. These results are expected, occurring as a consequence of epitaxial growth on an (001)-oriented $SrTiO_3$ substrate.

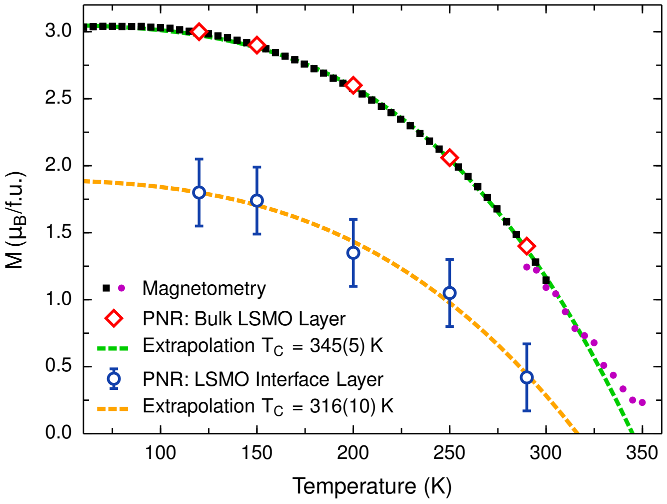


FIG. 4. Magnetometry provided an accurate magnetic moment of the bulk LSMO layer for fitting the temperature dependency PNR data measured on the instrument D3 in a magnetically saturated state (red diamonds). The fitted interface layer moment (blue circles) reveals a relatively constant depletion in percentage and layer thickness across the temperature range studied. An extrapolation of the data indicated a $T_C = 345(5)$ K of the bulk of the layer, and 316(10) K for the interfacial layer.

## III. POLARIZED NEUTRON REFLECTIVITY MODEL FITTING

The reflectometry data was fitted using the least squares refinement process. The $\chi^2$ residual-statistic commonly used in least squares refinement was not used for the minimization process, as it overrates reflectivity signals by over-weighting low-$Q_Z$ data points with high counting statistics, and underrates high-$Q_Z$ data points with low counting statistics. Instead, the residual-statistic used to determine the difference between the fitted model and experimental data was calculated using Eqn. (1), where $R_{exp}$ and $R_{sim}$ are the experimental and theoretical reflectivity intensities at momentum transfer $Q_Z$, respectively.

$$\text{residual statistic} \quad = \sum_{Q_{min}<Q_Z<Q_{max}} \left( \frac{R_{sim}(Q_Z) - R_{exp}(Q_Z)}{R_{sim}(Q_Z) + R_{exp}(Q_Z)} \right)^2 \tag{1}$$

Using (1), the residual-statistic is renormalized by the total reflection, and does not take the statistical error of the points into consideration. The $Q_Z$ range was 0.025–0.36 Å$^{-1}$ for the synchrotron X-ray reflectivity patterns, and 0.01–0.1 Å$^{-1}$ for the polarized neutron reflectivity patterns.

In order to visualize the stability of the obtained fitting minima that represent the most likely values of the fitting parameters, we present residuum stability plots in two-dimensional parameter space. Figure 5 plots the calculated residual-statistic as a function of the LSMO interfacial modification thickness and magnetic moment for data obtained by PNR on the NREX instrument. In Fig. 6, the residual-statistic is plotted as a function of the interfacial modification thickness and relative change in refractive index for the XRR data collected on the UE56/2-PGM1 beamline at BESSY-II at the Mn $L_3$ edge (644.1 eV). The overall thickness of the LSMO layer was kept constant while adjusting the interface thickness. Both plots indicate a single and stable minimum with the best fit parameters presented in the main text.

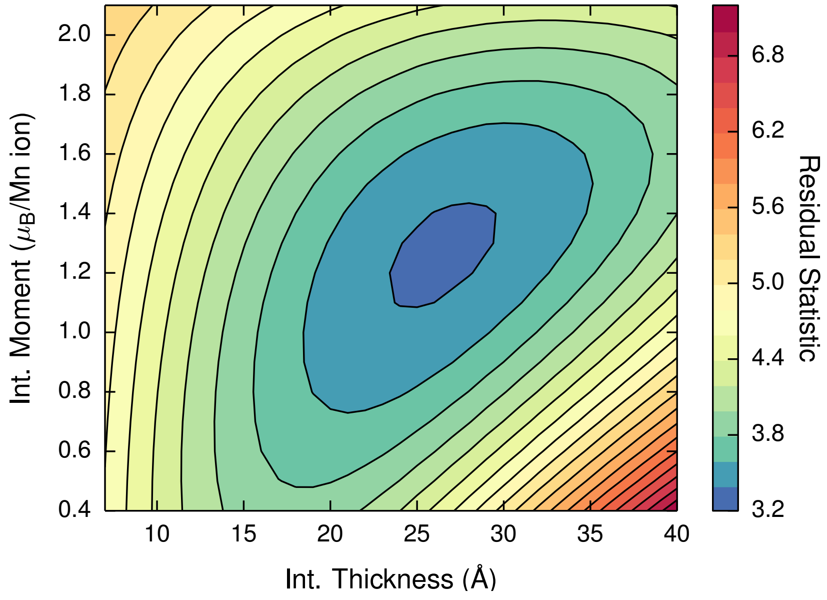


FIG. 5. Stability plot of the fit to the PNR data obtained on the NREX instrument, plotting the residual-statistic of the simulation model as described in the main text as a function of LSMO interface modification thickness and magnetic moment. Relates to Fig. 1 in the main text.

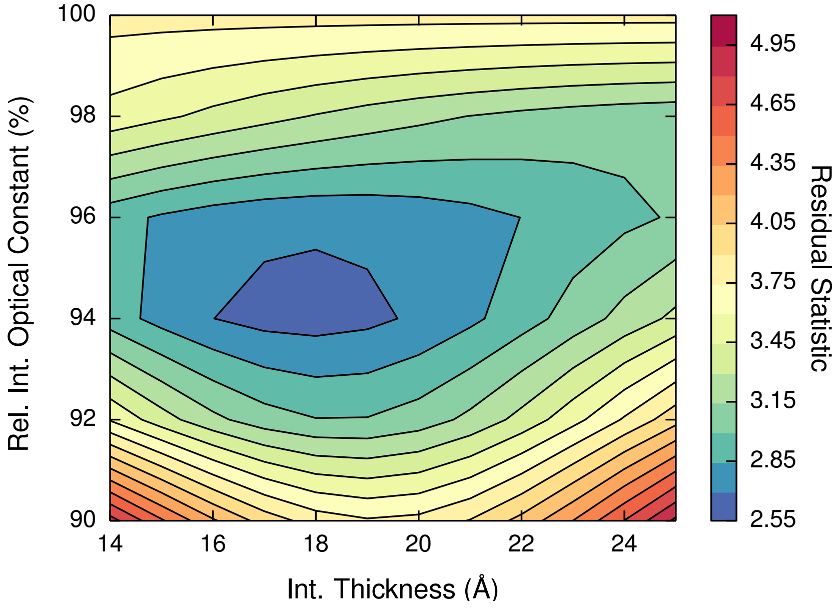


FIG. 6. Stability plot of the simulation fitting of the synchrotron XRR data obtained at BESSY-II at the Mn $L_3$ edge (644.1 eV). The optical constant is presented in terms of the relative change from the optical constant of the bulk of the LSMO layer. Relates to Fig. 4 in the main text.

[1] C. Kisielowski, *et al*. Microsc. Microanalysis **14**, 469-477 (2008).

[2] R.F. Egerton, Electron Energy-loss Spectroscopy in the Electron Microscope, Plenum Press (Springer), London, 2nd Edition (1996).

[3] M. Watanabe, E. Okunishi, and K. Ishizuka, Microsc. Anal. **23**, 5 (2009).

[4] A. B. Shah, Q. M. Ramasse, J. G. Wen, A. Bhattacharya, and J. M. Zuo, Micron **42**, 539 (2011).
